# Supplementary material for: FedRN: Exploiting k-Reliable Neighbors Towards Robust Federated Learning
Source: arXiv:2205.01310 source file (2022-09-19)
Supplement: Supplementary file 1 [file 8-appendix.tex]

% \section{Detailed Cost Analysis}
% \label{sec:cost_analysis}

% We analyze the communication and computation cost of \algname{} compared with other {six} methods, as summarized in Table \ref{tab:analysis-cost}.
% In this comparison, the communication cost is split into two parts, \enquote{server$\rightarrow$client} and \enquote{client$\rightarrow$server,} while the computation cost is split into two other parts, \enquote{forward} and \enquote{backward,} and the \enquote{total cost} aggregates all the costs for each perspective. 

% \input{tab-ablation-alpha}


% \begin{itemize}[leftmargin=*]
% \item \underline{Communication Cost:} \algname{} requires {3M} or {4M} communication cost in total when using one or two reliable neighbors, which is a sufficient number for general use cases. The remaining communication cost for calculating data similarity and expertise\,(i.e., $Acc({\sf c})$ and $p(\tilde{x};\Theta_{\sf c})$) is negligible. By contrast, Co-Teaching and DivideMix both require 4M communication cost in total because they maintain two models for co-training. In summary, \algname{} leads to greater performance with comparable or lower communication cost compared with other baseline methods.
% \smallskip

% \footnotetext[6]{If the number of clients is large, a large computation cost may be required to search the $k$-reliable neighbor. However, by using the \textit{KD-Tree algorithm}, the computation cost can be greatly reduced\,\cite{jeong2020federated}.}

% \item \underline{Computation Cost:} We exclude the cost of fitting GMMs and searching $k$-reliable neighbors\footnotemark[6] because their costs are negligible compared to those of the forward and backward steps. Along the pipeline of our local update phase, \algname{} first requires $k$F and $k$B computation cost to perform fine-tuning with $k$-reliable neighbors for one epoch. Next, to construct the clean set, $(k+1)$F communication cost is needed due to the inference with $k+1$ available models. As the constructed clean set is deterministic over all the local epochs, only $e$F+$e$B computation cost is required to train a single model for the given local epoch $e$ in each communication round. Consequently, \algname{} needs $(e+2k+1)$F + $(k+e)$B computation cost in total. 
% %
% In a typical deep learning pipeline, the cost of the backward step is relatively smaller than that of the forward step. Hence, the computation cost for the forward step is the major issue. In light of this fact, the forward cost of \algname{} is comparable to those of FedAvg, Joint-optim, and SELFIE, and less than those of Co-teaching and DivideMix, because the number of local epochs is larger than the number of reliable neighbors, $e > k$. Among the compared methods, DivideMix is the slowest method in that it performs $m$ data augmentations with two models for each local epoch, so its forward cost is $(4m+2)e$F. 
% \end{itemize}

% Therefore, with one or two reliable neighbors, \algname{} greatly improves the robustness of the global model without adding much communication and computation cost in the scenario of federated learning with noisy labels.



% A. Experiment Configuration Details
% A.1. Datasets
% A.2. Hyperparameters

% B. Supplementary Evaluation
% B.1. Comparison with $k$-Random Neighbors.
% B.2. Effect of \# Neighbors

% C. Discussion
% C.1. Model Aggregation with Reliablity Score
% C.2. Dynamic Alpha
% C.3. w. Semi-sup

% \section{A ~~Experiment Configuration Details}
% In this section, we specify the details of our experiment configuration concerning datasets and hyperparameters.% about other baseline methods. 

% %\subsection{A.1 ~~ Datasets.}3
% \smallskip
% \noindent\textbf{Datasets.}
% %To verify the performance of \algname{}, 
% We used three synthetic or real-world benchmark datasets, two CIFAR datasets\footnote{\url{https://www.cs.toronto.edu/~kriz/cifar.html}}, and mini-WebVision\footnote{\url{https://data.vision.ee.ethz.ch/cvl/webvision/dataset2017.html}}. 
% % The statistics for the three datasets are summarized in Table \ref{tab:summary_data}. 

% % \input{tab-summary-data}



%\subsection{A.2 ~~ Hyperparameters about Baseline Methods}
% \noindent\textbf{Algorithm Hyperparamters.}
% For reproducibility, we clarify the hyperparmeter setup of all baseline algorithms.
% \begin{itemize}[leftmargin=*]
% \item Joint Optimization: The loss function consists of a classification loss and two regularization losses. These two regularization losses are adjusted with the hyper parameters $\alpha$ and $\beta$. We set these $\alpha$ and $\beta$ to 1.2 and 0.8, respectively.
% \item SELFIE: The uncertainty threshold $\epsilon$ and label history for each sample are required for training. As suggested in the paper, we set the uncertainty threshold $\epsilon$ and history size $q$ to 0.5 and 15, respectively.
% \item DivideMix: DivideMix applies MixMatch for semi-supervised learning. Dividemix uses hyperparameters for MixMatch such as a sharpening temperature $T$, unsupervised loss weight $\lambda_u$, Beta distribution parameter $\alpha$. We set $T$, $\lambda_u$, and $\alpha$ to 0.5, 25, and 4, respectively.
% \end{itemize}
%For Joint Optimization, the loss function consists of a classification loss and two regularization losses. These two regularization losses are adjusted with the hyper parameters $\alpha$ and $\beta$. We set these $\alpha$ and $\beta$ to 1.2 and 0.8, respectively. For SELFIE, the uncertainty threshold ($\epsilon$) and label history for each sample are required for training. As suggested in the paper, we set the uncertainty threshold($\epsilon$) and history size ($q$) to 0.5 and 15, respectively. DivideMix applies MixMatch for semi-supervised learning. Dividmix uses hyperparameters for MixMatch such like sharpening temperature $T$, unsupervised loss weight $\lambda_u$, Beta distribution parameter $\alpha$. We set $T$, $\lambda_u$, and $\alpha$ to 0.5, 25, and 4, respectively.
%\smallskip
%\noindent\textbf{Development Environment.}
%All of the algorithms were implemented using PyTorch $1.7.0$ and executed using four NVIDIA RTX 2080Ti GPUs. 




%\section{Supplementary Evaluation}

% \section{Grid Search for Balancing Term $\alpha$} 
% \label{sec:parameter_search}

% We adjusted $\alpha$ to determine the contribution of data expertise and similarity in neighbor search. To ascertain the optimal value, we repeated the experiment on CIFAR-10 with various $\alpha$ values, as summarized in Table \ref{tab:ablation-alpha}. Because the fine-tuning technique is incorporated in \algname{}, merging data expertise and similarity provides a synergistic enhancement in general. In particular, when $\alpha = 0.6$, the performance gain is the highest on average. 
% Based on the two studies on our hyperparameters, we set $\alpha$ to $0.6$ for all experiments in Section \ref{sec:evaluation}.

% \input{tab-ablation-random}

% \section{Comparison with Random Neighbors\!\!\!\!\!}
% \label{sec:random_analysis}

% % We further show $k$-reliable neighbors are much useful than $k$-random neighbors for overcoming the performance discrepancy over clients. 
% %We emphasize the importance of reliability in consideration of the similarity of data distribution to the target client and expertise in labeling. 
% We analyzed the usefulness of $k$-reliable neighbors compared with $k$-random neighbors. For $k$-random neighbors, we replaced Lines 6 and 10 of Algorithm \ref{alg:fedrn} with random client selection.
% %
% %In this regard, we compared the performance with random neighbors that do not consider expertise and similarity. 
% Table \ref{tab:ablation-random} summarizes the test accuracy of \algname{} with $k$-reliable and $k$-random neighbors. 
% Since our fine-tuning technique was incorporated with $k$-random neighbors, using $k$-random neighbors improves the robustness against noisy labels, but \algname{} with $k$-reliable neighbors maintains its dominance in every case.
% %The random neighbors can also derive somewhat comparable performance through fine-tuning using target client data. 
% In detail, if the neighbors with low data expertise are selected, they misclassify mislabeled examples as clean examples in sample selection. Likewise, the neighbors with significantly different data distributions harm identifying clean examples from the target client’s noisy data due to the distribution shift problem. It can be confirmed experimentally that this issue becomes more prominent when the noise rate is high. In conclusion, we should leverage the reliability of neighbors to obtain a global model robust to noisy labels.


% \section{Detailed Convergence Curves}
% % Main에 옮기고 convergence 이슈가 없음을 강조
% \label{subsect:performance_analysis}

% Figure \ref{fig:train_test_acc} shows the convergence curves on the training and test accuracy during all the training rounds. In our experimental configuration, the global model of all methods is observed to converge in training and test accuracy. Overall, FedRN shows outstanding test accuracy compared with other robust methods. However, Joint-optimization and Robust FL show poor performance because they produce many false corrections in the re-labeling process. Particularly, in a Non-IID learning scenario with noisy labels, the probability of mislabeling is prone to be very high due to the low-performing global model. As a result, their training and test accuracy decline drastically immediately after the warm-up period at the $100$th training round. In contrast, the remaining robust methods including \algname{} show better convergence curves than FedAvg because the model is updated only 
% with the selected clean examples after the warm-up period. \looseness=-1

% \begin{figure*}[b!]
% \begin{center}
% \subfloat[CIFAR-10 ($S=2$) with symmetric noise 0.0--0.4]{\includegraphics[width=17.0cm]{figures/evaluation/acc_cifar10_sym40.pdf}}
% \vspace*{0.4cm}
% \subfloat[CIFAR-10 ($S=2$) with symmetric noise 0.0--0.8]{\includegraphics[width=17.0cm]{figures/evaluation/acc_cifar10_sym80.pdf}}
% \vspace*{0.4cm}
% \subfloat[CIFAR-100 ($S=20$) with symmetric noise 0.0--0.4]{\includegraphics[width=17.0cm]{figures/evaluation/acc_cifar100_sym40.pdf}}
% \end{center}
% \vspace*{-0.4cm}
% \caption{Convergence curves of training and test accuracy for CIFAR-10 and CIFAR-100}
% \label{fig:train_test_acc}
% \vspace*{0.15cm}
% \end{figure*}


% \begin{figure}
%     \captionsetup[subfloat]{margin=10pt,format=hang,singlelinecheck=false,justification=RaggedRight}
%     \centering
%     \subfloat[line break should \protect\\ be here]{\includegraphics[scale=0.5]{example-image-a}}

%     \subfloat[newline \newline
%     there]{\includegraphics[scale=0.5]{example-image-a}}
%     \caption{Test figure.}
% \end{figure}
