# Supplementary material for: FedRN: Exploiting k-Reliable Neighbors Towards Robust Federated Learning
Source: arXiv:2205.01310 source file (2022-09-19)
Supplement: Supplementary file 2 [file tab-cifar10-appendix.tex]

{
\newcolumntype{L}[1]{>{\raggedright\let\newline\\\arraybackslash\hspace{0pt}}m{#1}}
\newcolumntype{X}[1]{>{\centering\let\newline\\\arraybackslash\hspace{0pt}}p{#1}}
\begin{table*}[!t]
\caption{Test accuracy\,(\%) on CIFAR-10 with symmetric, asymmetric\,(Asym), and mixed noise\,(Mixed).}
%\small
\vspace*{-0.3cm}
\begin{tabular}{L{2.2cm} |X{0.91cm}X{0.91cm}|X{0.91cm}|X{0.91cm}|X{0.91cm}X{0.91cm}|X{0.91cm}|X{0.91cm}|X{0.91cm}X{0.91cm}|X{0.91cm}|X{0.91cm}}\toprule
Non-IID Type &  \multicolumn{4}{c|}{Shard\,($S=2$)} & \multicolumn{4}{c|}{Shard\,($S=5$)} & \multicolumn{4}{c}{Dirichlet\,($\beta=0.5$)}  \\\midrule
Noise Type & \multicolumn{2}{c|}{Symmetric} & {Asym} & {Mixed} & \multicolumn{2}{c|}{Symmetric} & {Asym} & {Mixed} & \multicolumn{2}{c|}{Symmetric} & {Asym} & {Mixed} \\
Noise Rate & \!\!0.0--0.4\!\! & \!\!0.0--0.8\!\! & \!\!0.0--0.4\!\! & \!\!0.0--0.4\!\! & \!\!0.0--0.4\!\! & \!\!0.0--0.8\!\! & \!\!0.0--0.4\!\! & \!\!0.0--0.4\!\! & \!\!0.0--0.4\!\! & \!\!0.0--0.8\!\! & \!\!0.0--0.4\!\! & \!\!0.0--0.4\!\! \\\toprule
Oracle\footnotemark[3]     & 69.10 & 67.19 & 69.10 & 68.89 & 78.00 & 75.94 & 78.00 & 77.7 & 81.79 & 80.38 & 81.79 & 81.39 \\ \midrule
FedAvg\,\cite{mcmahan2017communication}     & 46.39 & 38.69 & 49.09 & 46.82 & 66.44 & 56.46 & 67.23 & 67.95 & 75.92 & 70.60 & 77.77 & 77.17 \\
Co-teaching\,\cite{han2018co}\!\! & 63.20 & 52.72 & 62.48 & 61.68 & 74.66 & 67.17 & 74.18 & 75.18 & 79.97 & 75.39 & 79.53 & 79.94 \\
Joint-optm\,\cite{tanaka2018joint}  & 50.44 & 42.23 & 38.04 & 47.28 & 69.22 & 64.02 & 67.29 & 68.84 & 75.46 & 70.43 & 74.81 & 75.43 \\
SELFIE\,\cite{song2019selfie}      & 62.64 & 53.69 & 64.21 & 62.63 & 74.57 & 66.90 & 74.77 & 74.44 & 78.57 & 72.92 & 78.58 & 79.02 \\
DivideMix\,\cite{li2020dividemix}   & 62.35 & 58.18 & 62.07 & 63.38 & 68.73 & 65.82 & 68.95 & 69.32 & 74.26 & 72.25 & 73.29 & 73.47 \\  
Robust FL\,\cite{yang2020robust} & 56.25 & 45.59 & 55.52 & 57.58 & 70.30 & 62.89 & 69.04 & 70.02 & 75.75 & 70.63 & 74.00 & 75.49 \\
\midrule
\textbf{\algname{} (k=1)}  & 67.33 & 62.53 & \textbf{68.92} & \textbf{68.35} & 76.37 & 72.30 & 76.74 & 76.92 & 79.99 & 76.08 & 80.05 & 79.79 \\
\textbf{\algname{} (k=2)} & \textbf{67.62} & \textbf{62.94} &  67.51 & 66.91 & \textbf{76.81} & \textbf{72.85} & \textbf{77.33} & \textbf{76.99} & \textbf{80.34} & \textbf{76.49} & \textbf{80.38} & \textbf{80.28} \\

\bottomrule
\end{tabular}
\vspace*{-0.0cm}
\label{tab:cifar10-appendix}
\vspace*{-0.2cm}
\end{table*}
}
